# Supplementary material for: A Study of the Magnetic Activity and Variability of GJ 436
Source: arXiv:2209.11258 source file (2022-09-22)
Supplement: Supplementary file 1 [file Supplementary_Online_Material_File.pdf]

# Supplementary Online Material for 'A Study of the Magnetic Activity and Variability of GJ 436'

Mukul Kumar & Rim Fares

## 1 Activity Index Time Series for HARPS & NARVAL datasets

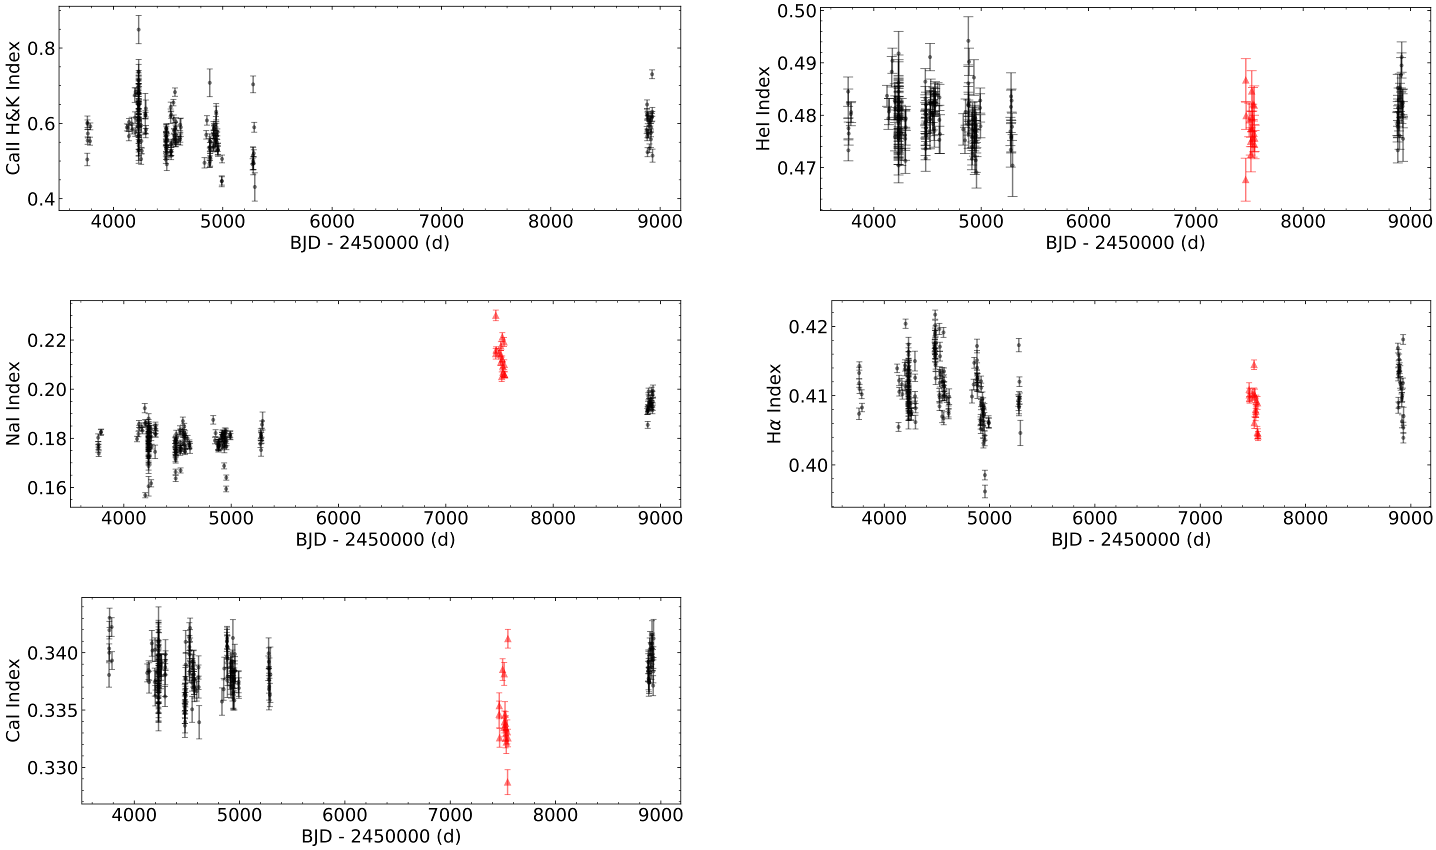


Figure 1: CaII H&K, HeI, NaI, H$\alpha$ & CaI activity indices of both HARPS and NARVAL datasets plotted against the BJD in one plot. The black dot markers are the HARPS indices and the black triangle markers are the NARVAL indices. The plot of CaII H&K indices does not include the NARVAL dataset since we calculated a CaII H index for it instead. The corresponding error bars for each index is plotted as well.

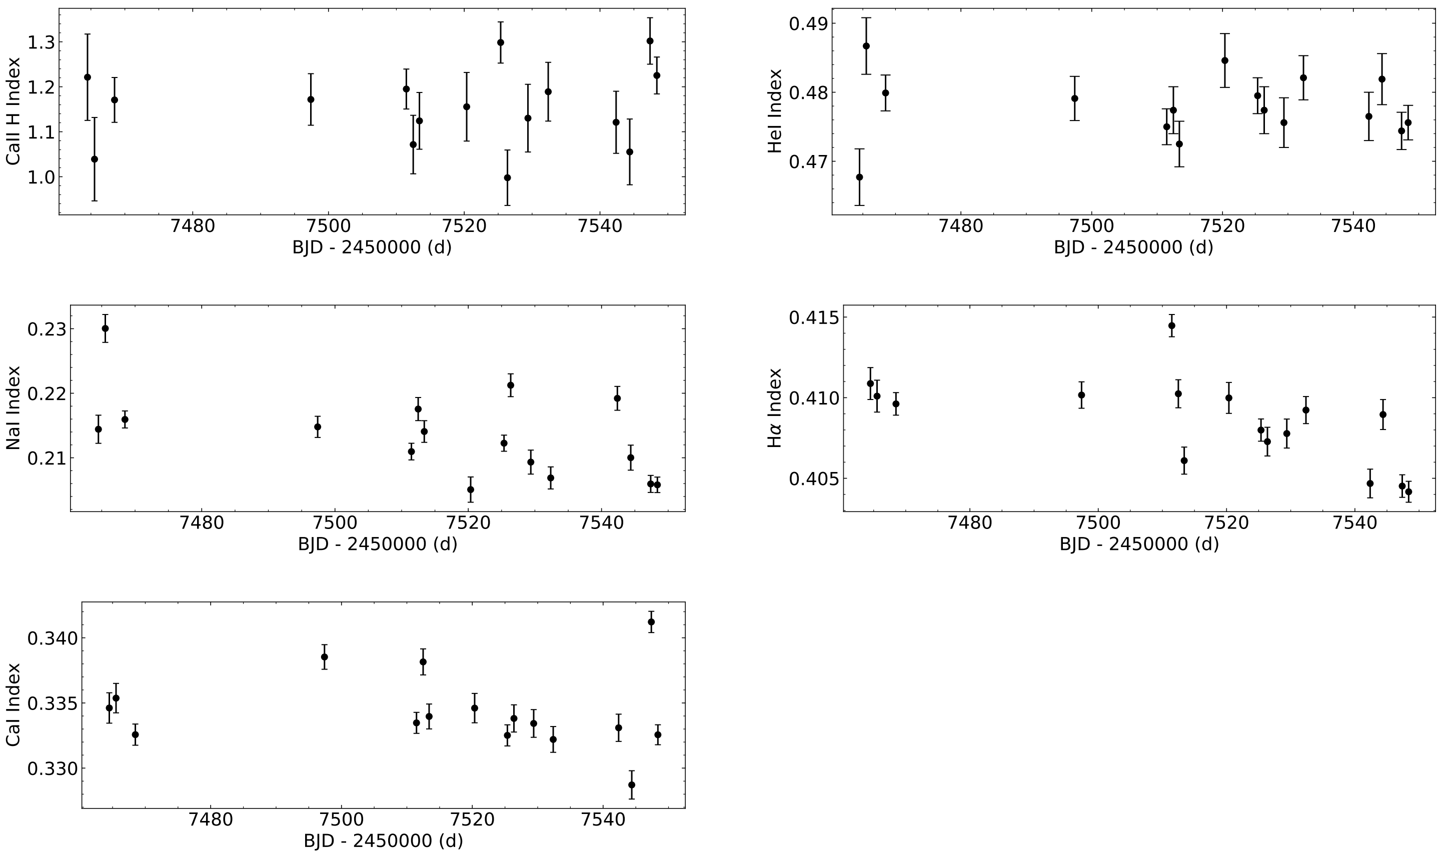


Figure 2: CaII H&K, HeI, NaI, H$\alpha$ & CaI activity indices calculated for the NARVAL dataset plotted against the BJD. These indices span $\approx 2$ stellar rotations, representing stellar short-term variations. The corresponding error bars for each index is plotted as well.

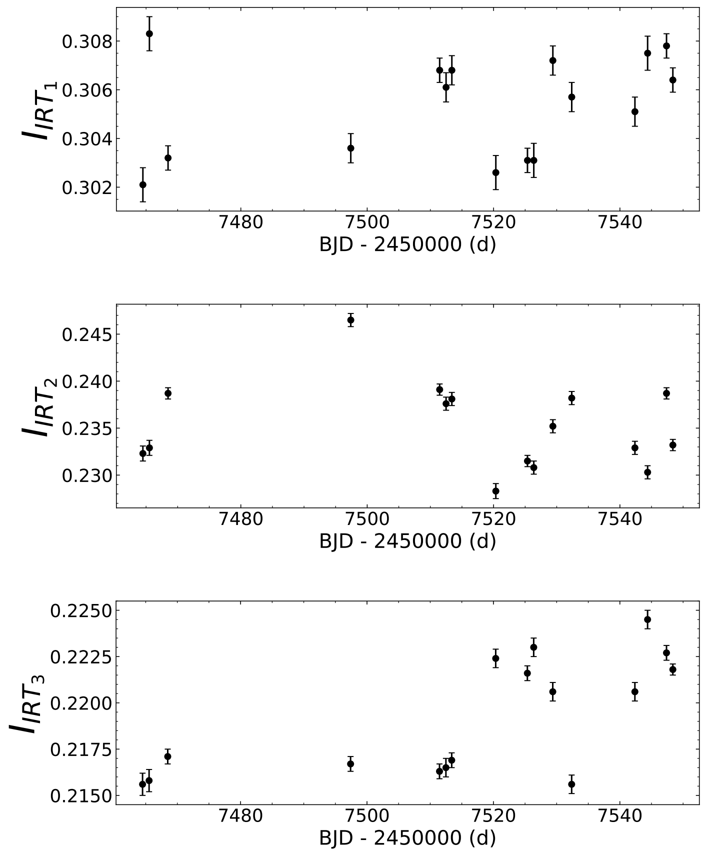


Figure 3: CaII IRT 1, IRT 2 & IRT 3 activity indices calculated for the NARVAL dataset plotted against the BJD. The corresponding error bars for each index is plotted as well.

## 2 Corner Plots showing Index Correlations per Observing Epoch

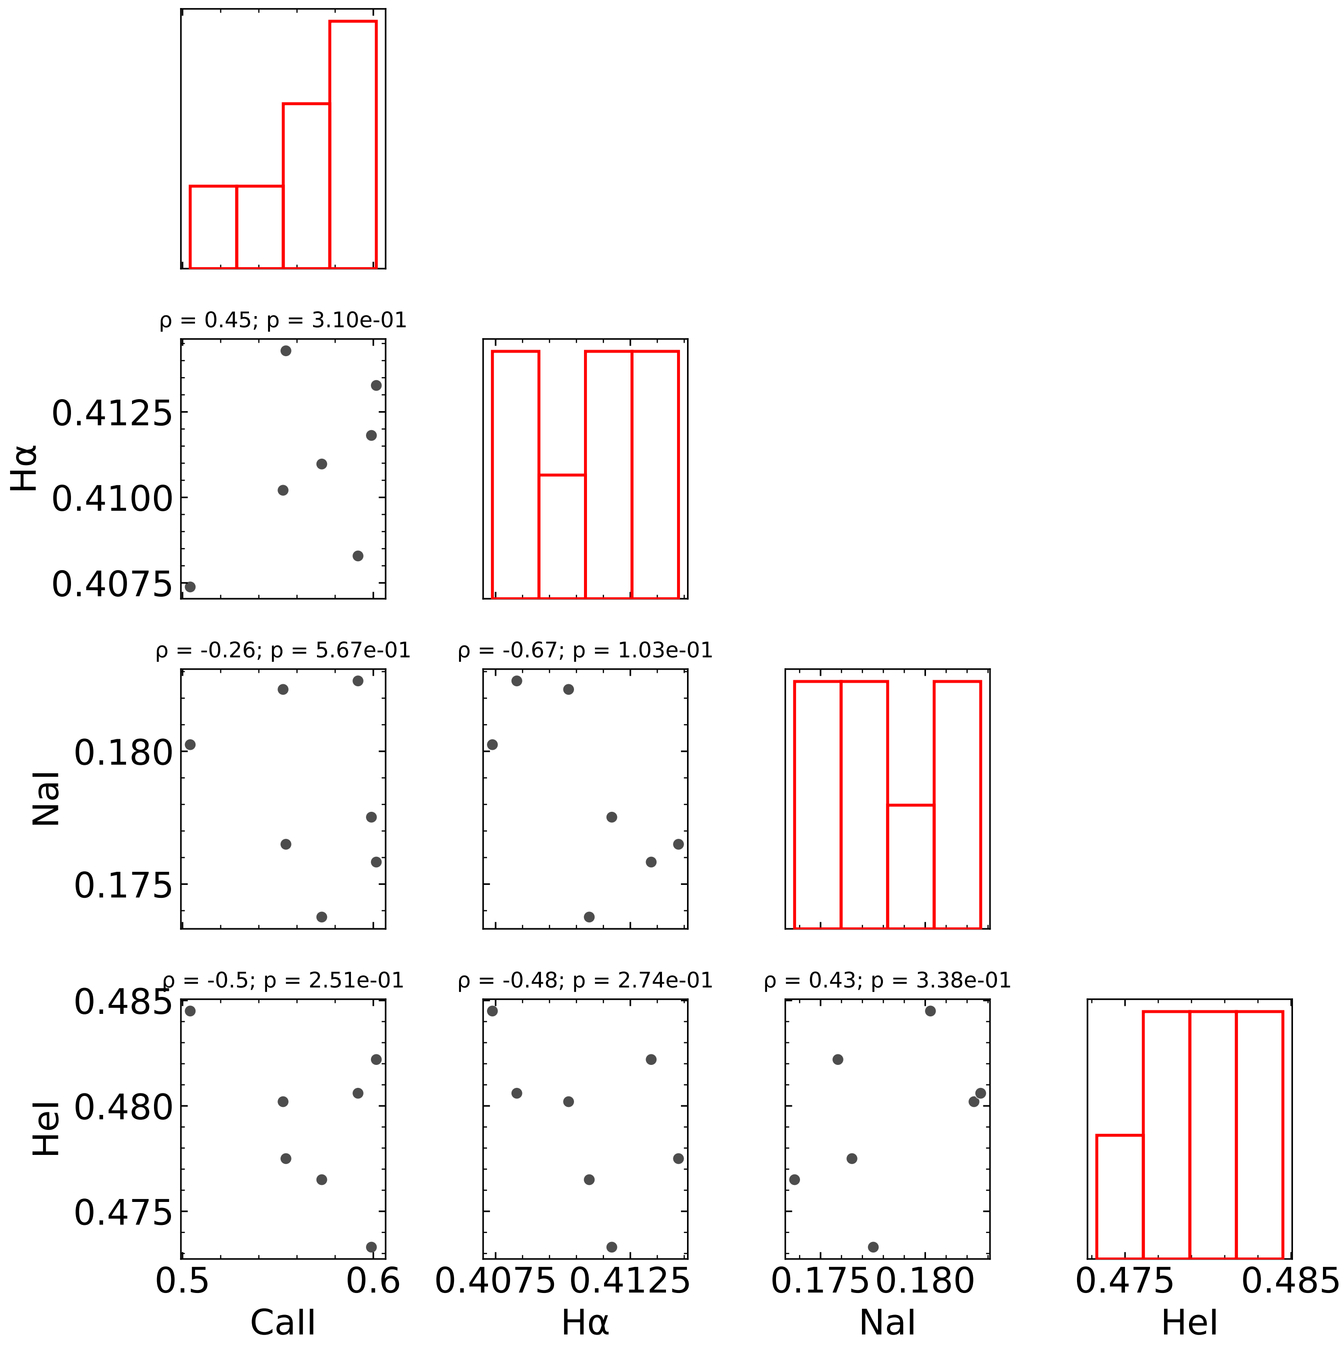


Figure 4: Corner plot showing correlations between the four activity indices CaII H&K, HeI, NaI and H$\alpha$, for 7 HARPS spectra in the 2006 observing epoch. The diagonal panels show the histogram distribution of each index. The Pearson R correlation coefficient ($\rho$) and its p-value are shown above each correlation plot, with significant correlation values shown in bold.

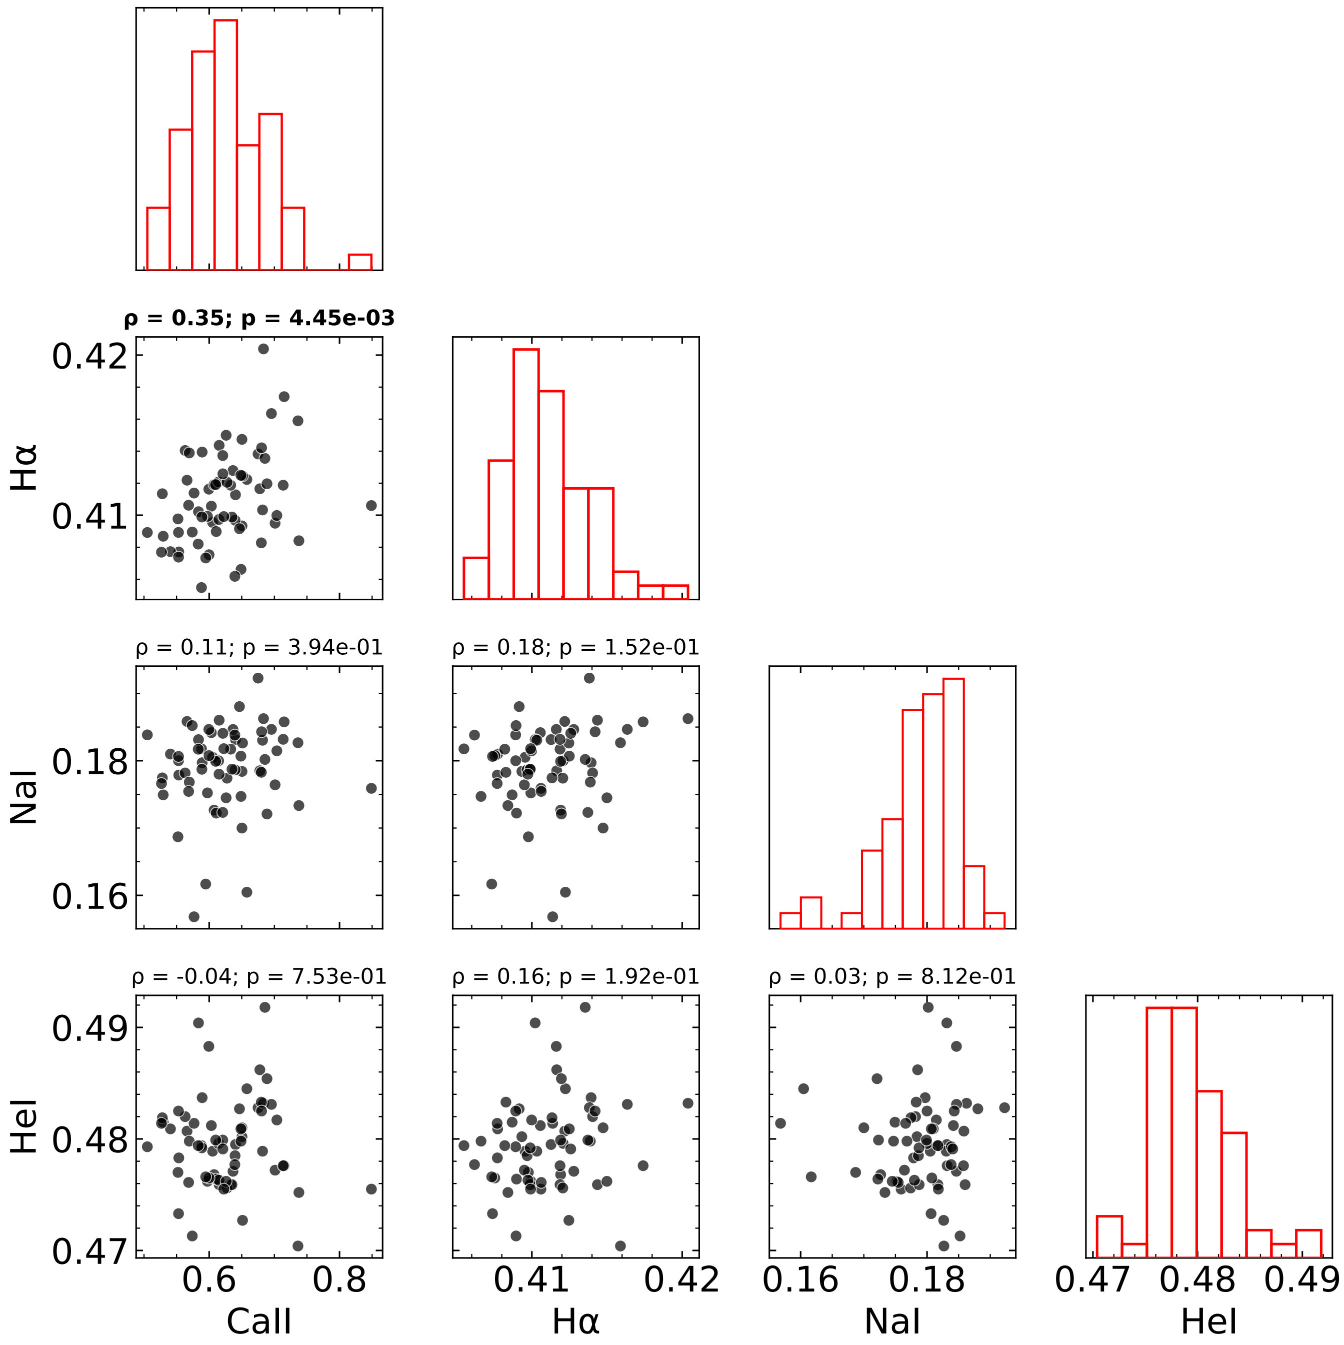


Figure 5: Same as figure 4 for 66 HARPS spectra in the 2007 observing epoch.

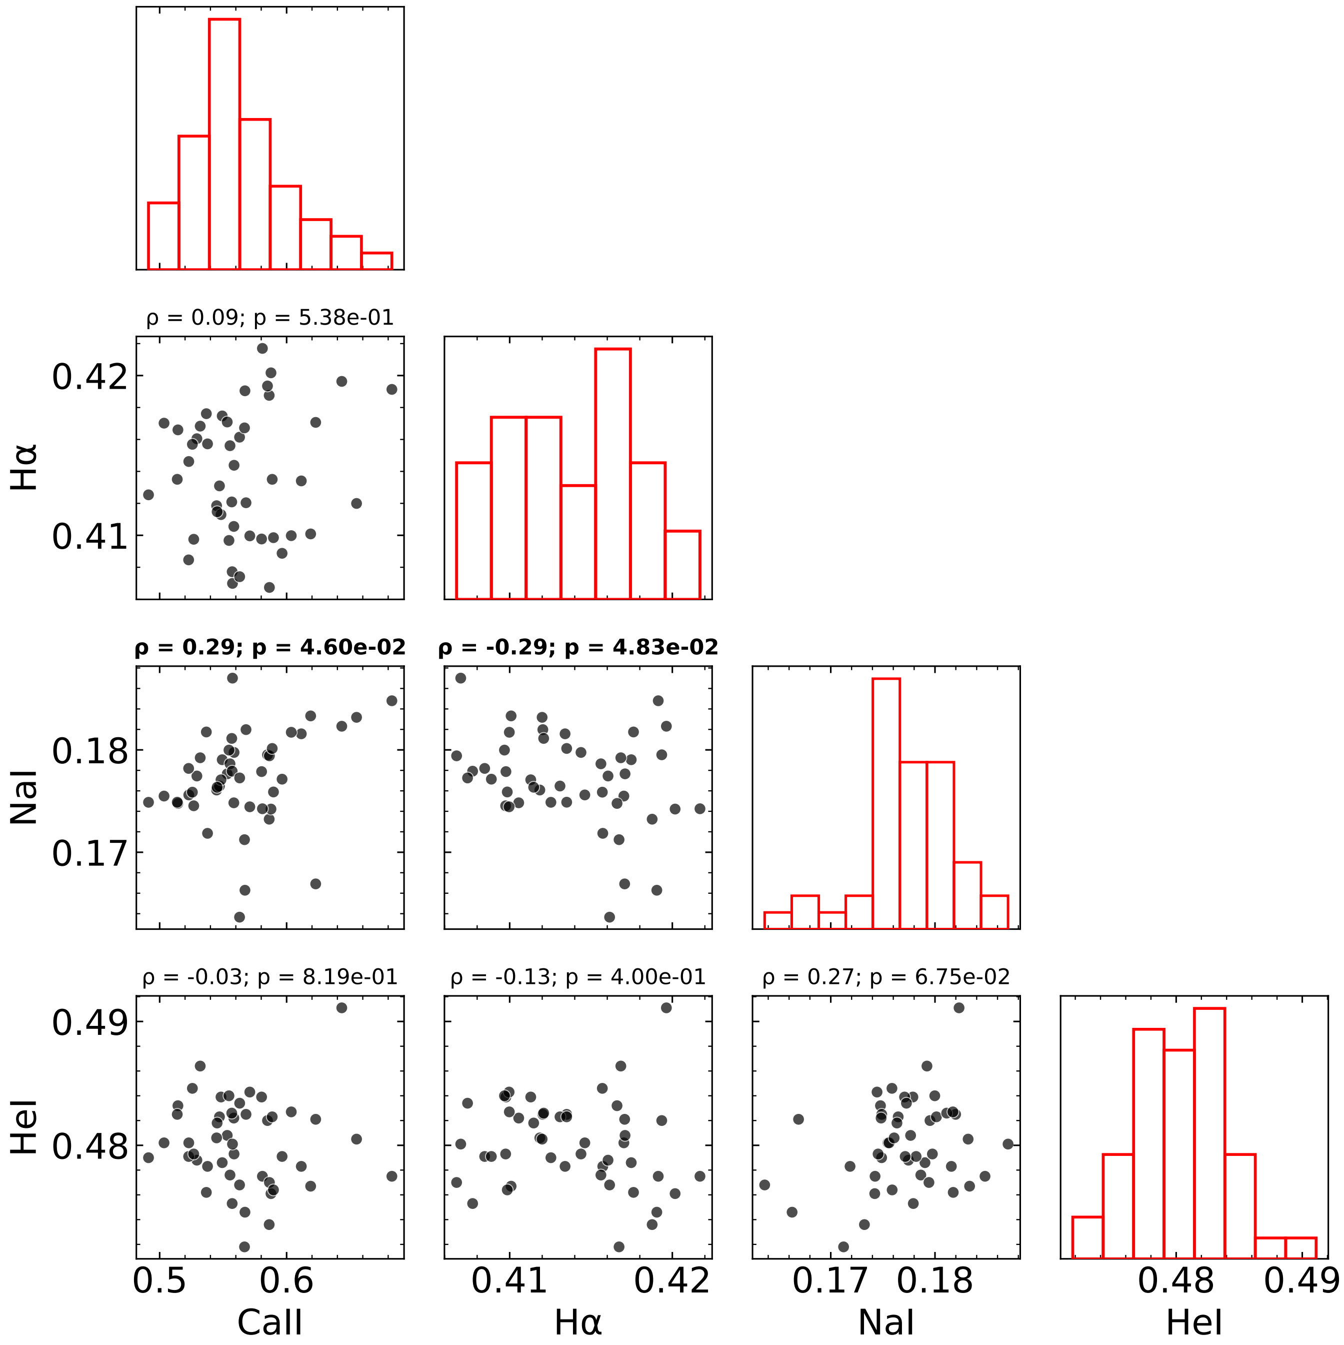


Figure 6: Same as figure 4 for 47 HARPS spectra in the 2008 observing epoch.

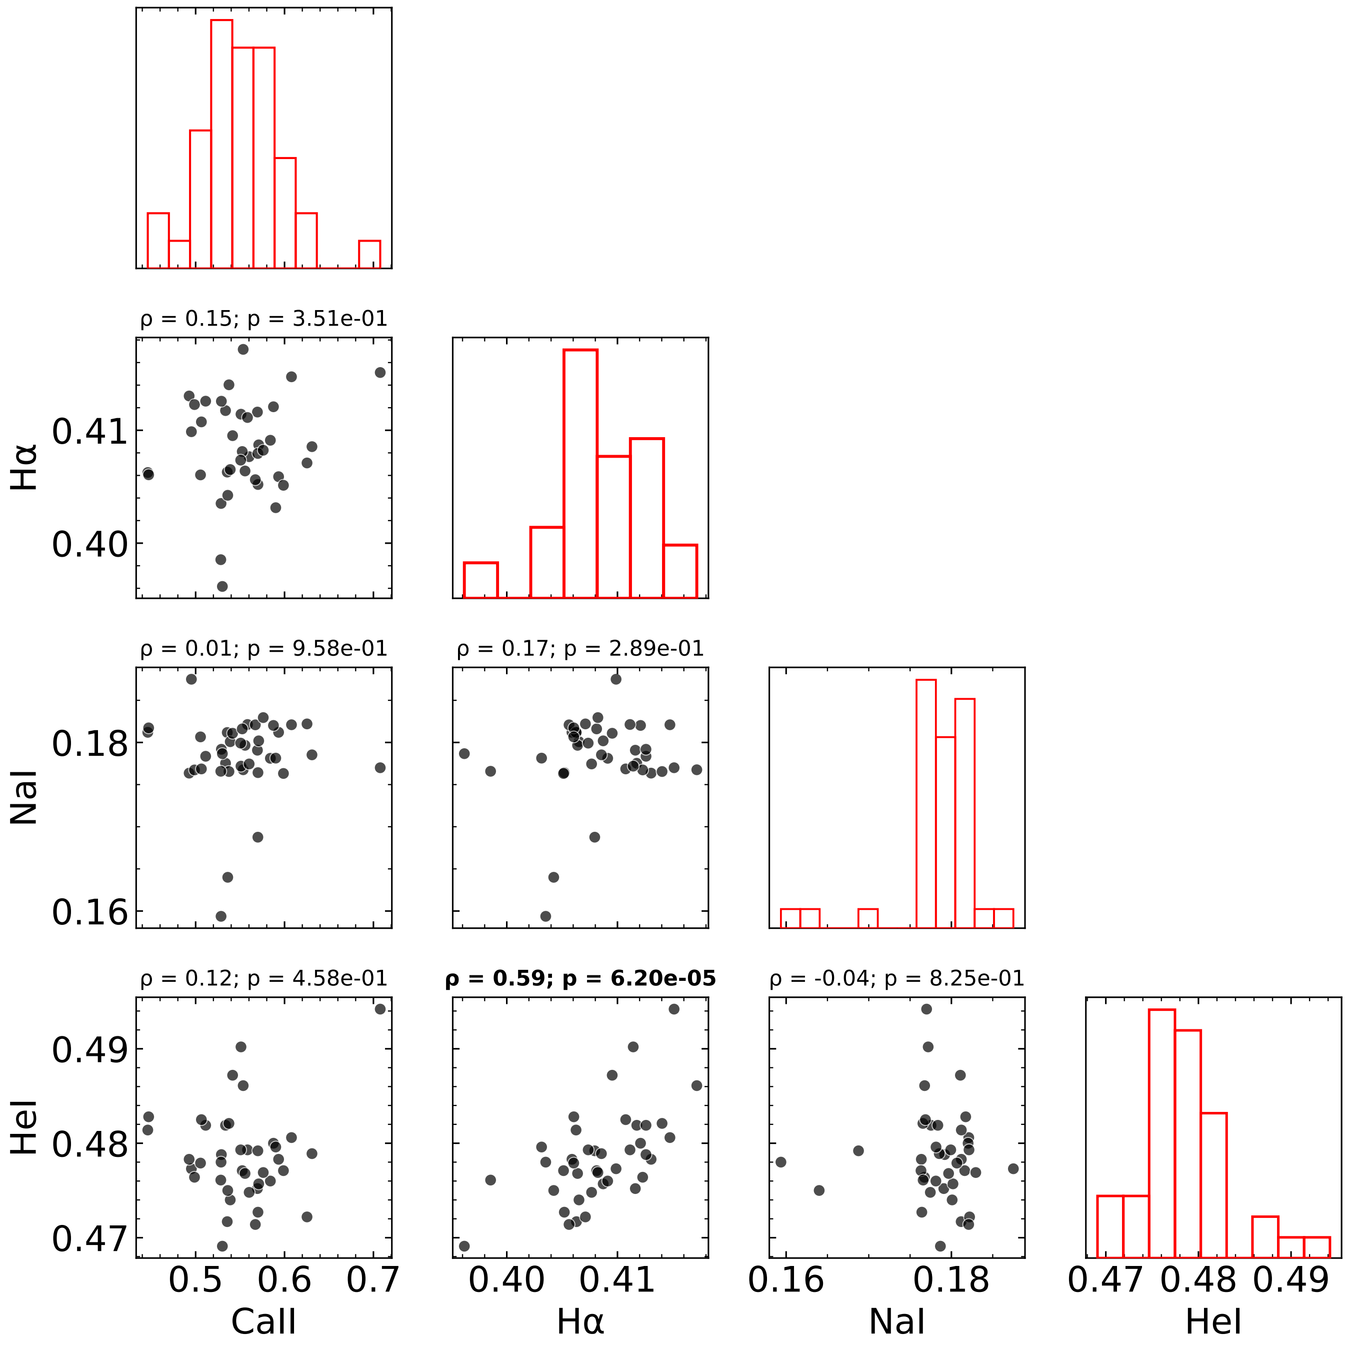


Figure 7: Same as figure 4 for 40 HARPS spectra in the 2009 observing epoch.

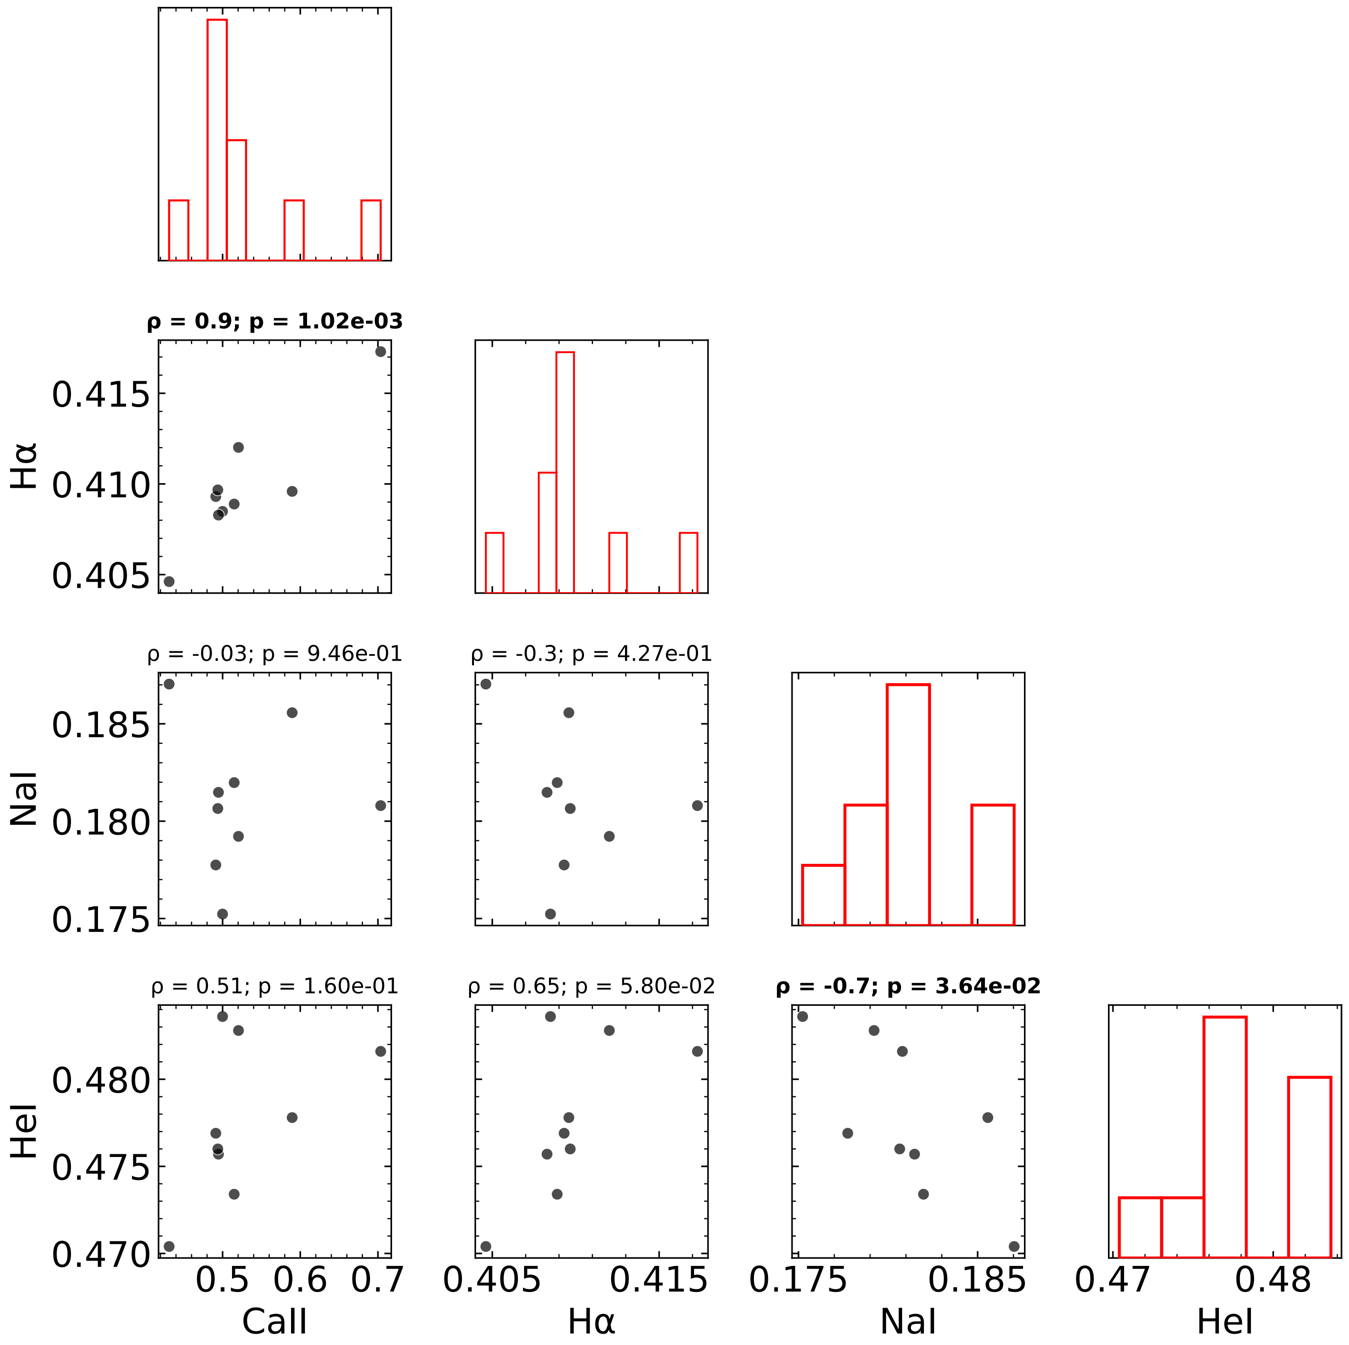


Figure 8: Same as figure 4 for 9 HARPS spectra in the 2010 observing epoch.

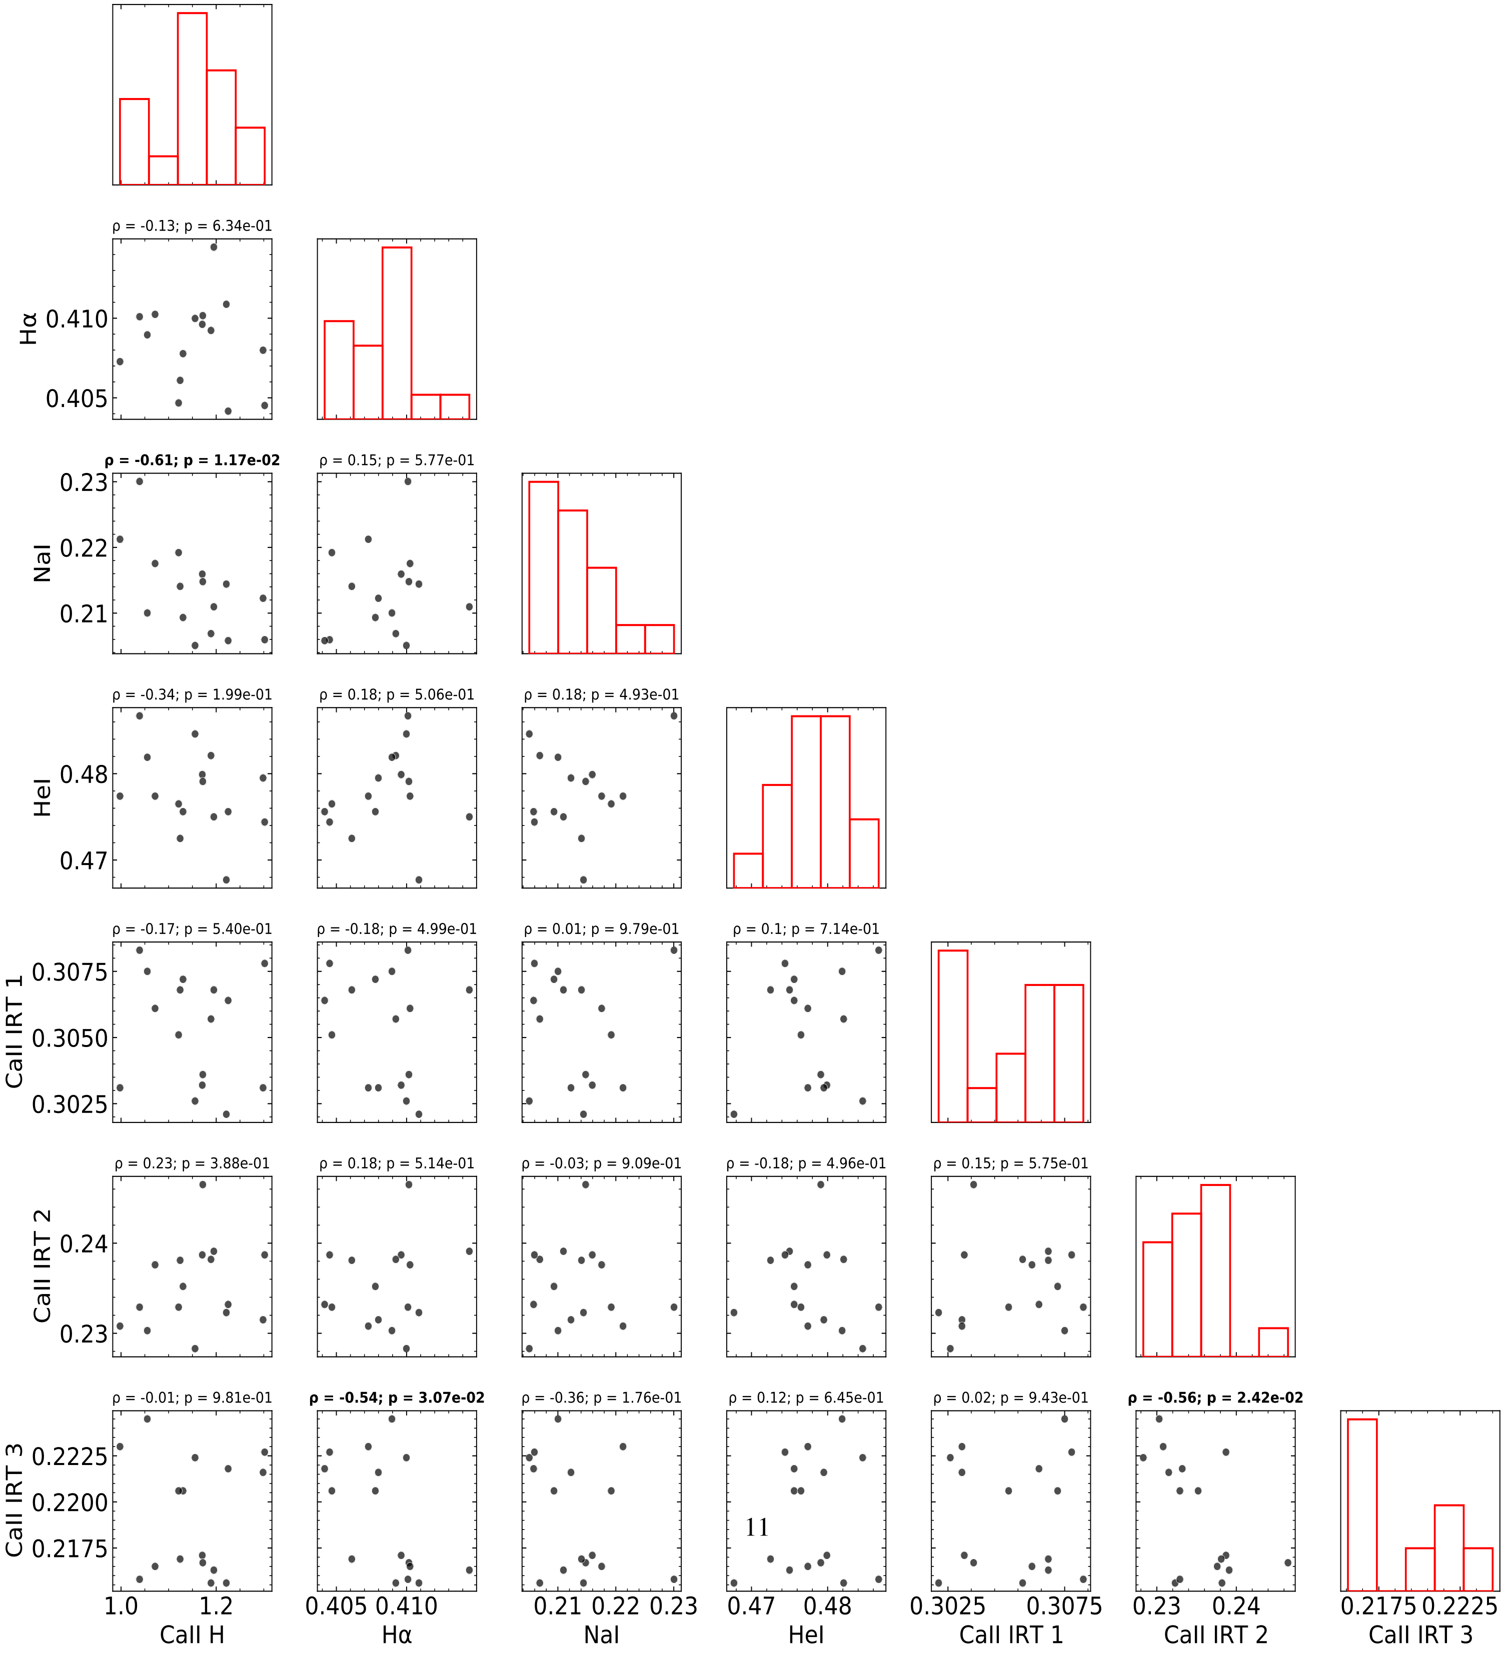


Figure 9: Same as figure 4 including the CaII infrared triplet (IRT) indices calculated for 16 NARVAL spectra in the 2016 observing epoch.

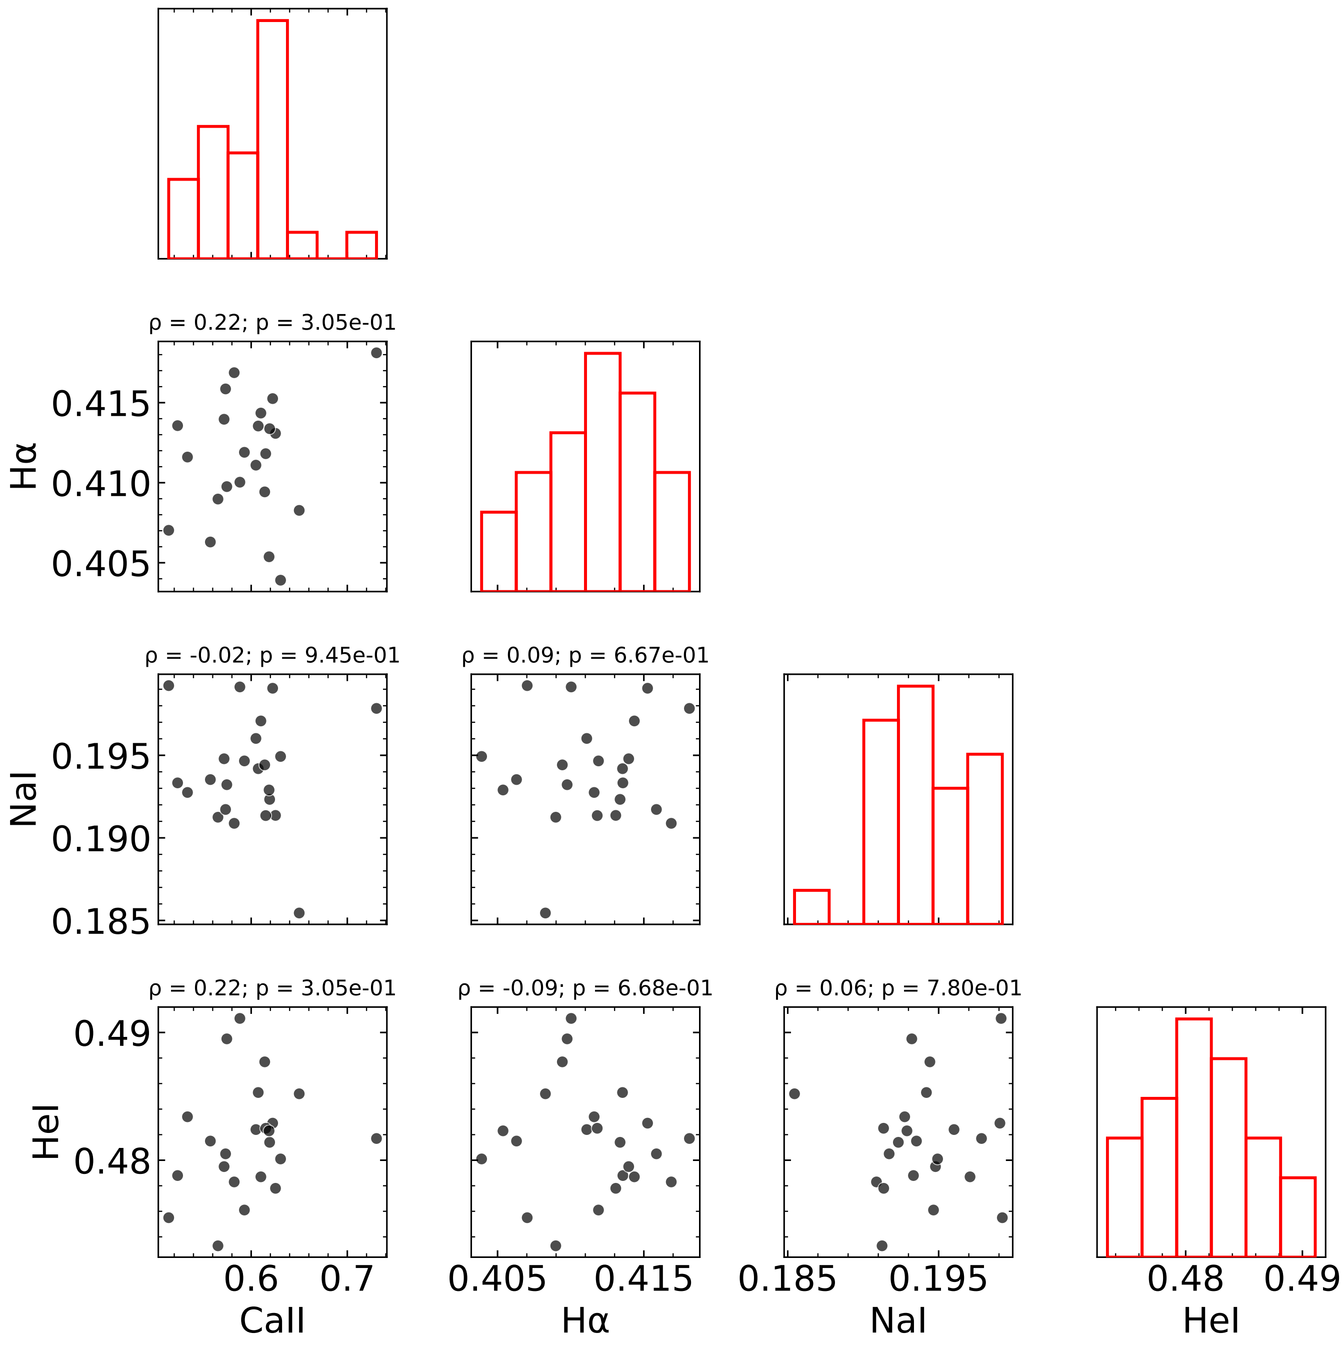


Figure 10: Same as figure 4 for 23 HARPS spectra in the 2020 observing epoch.

## 3 GLS Periodograms per Observing epoch for CaII H&, HeI, NaI & H$\alpha$ indices

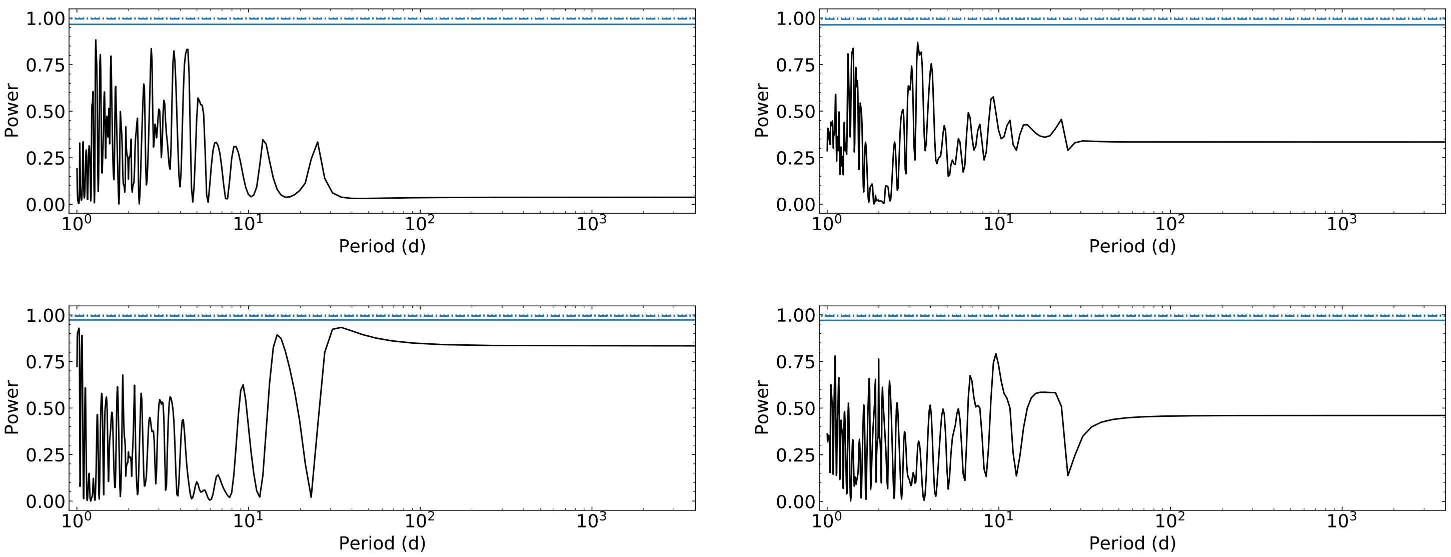


Figure 11: GLS periodogram of the CaII H&K (top left), HeI (top right), NaI (bottom left) and H$\alpha$ (bottom right) indices for 7 HARPS spectra in the 2006 observing epoch with the x-axis showcasing the trial periods in logarithmic scale. Detected periods are shown using appropriate coloured vertical lines with their respective periods mentioned in the plot legend of each periodogram. The solid, dash-dot and dotted blue horizontal lines show the false alarm levels for 10%, 1% and 0.1% respectively.

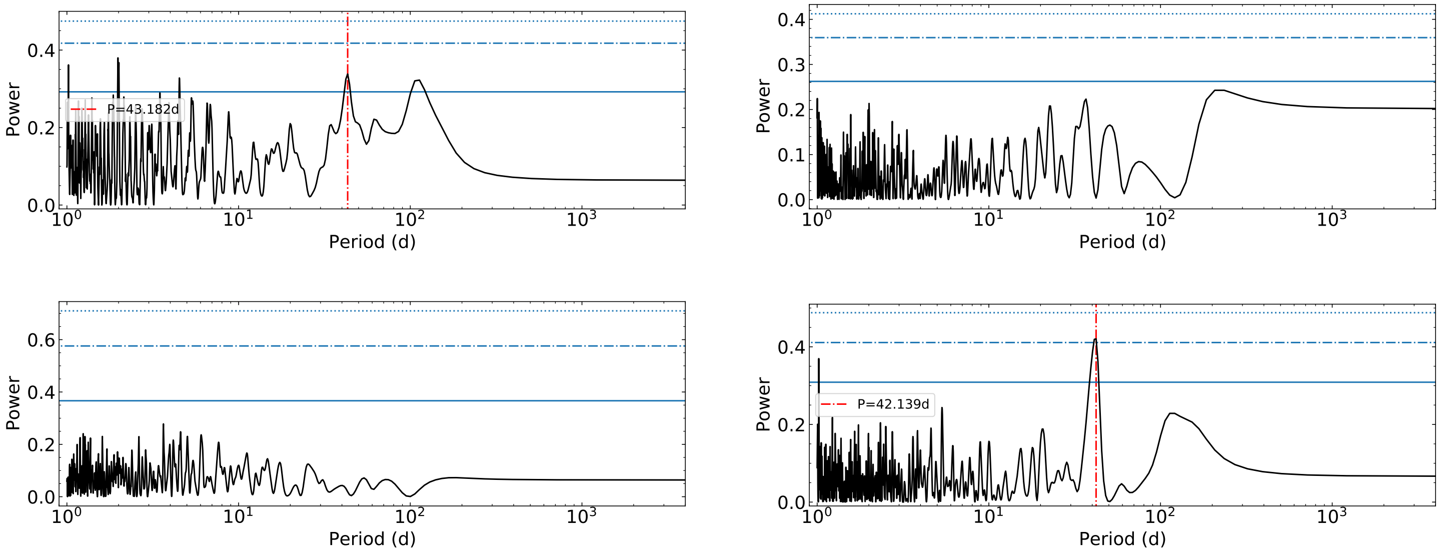


Figure 12: Same as figure 11 for 66 HARPS spectra in the 2007 observing epoch.

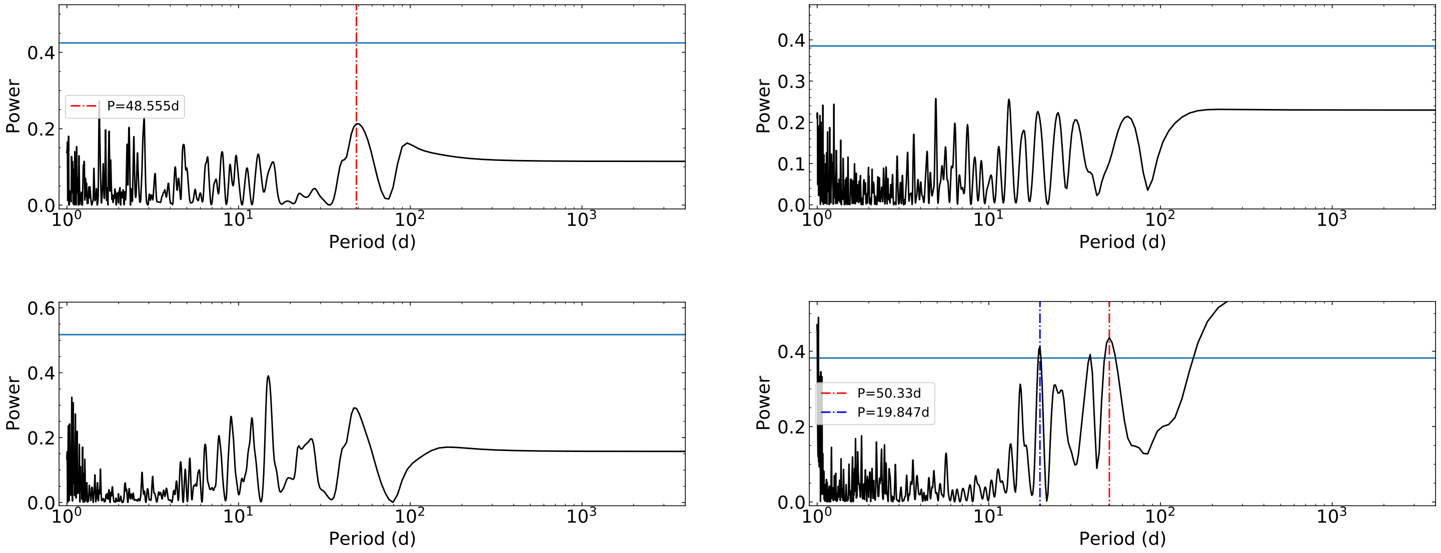


Figure 13: Same as figure 11 for 47 HARPS spectra in the 2008 observing epoch.

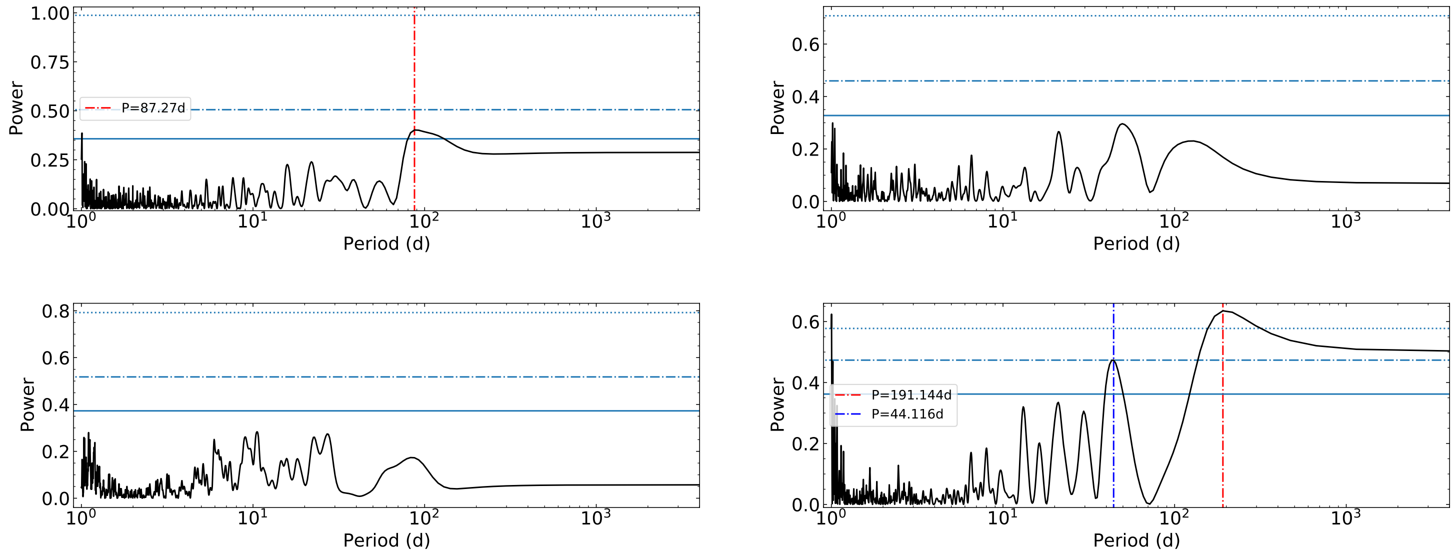


Figure 14: Same as figure 11 for 40 HARPS spectra in the 2009 observing epoch.

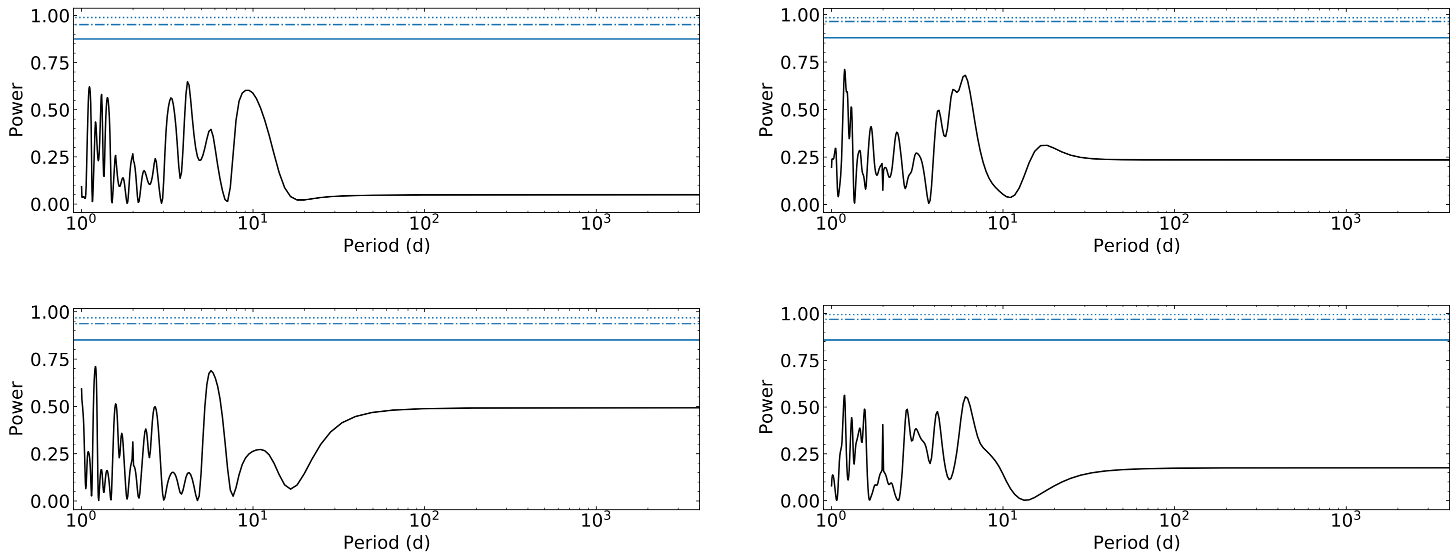


Figure 15: Same as figure 11 for 9 HARPS spectra in the 2010 observing epoch.

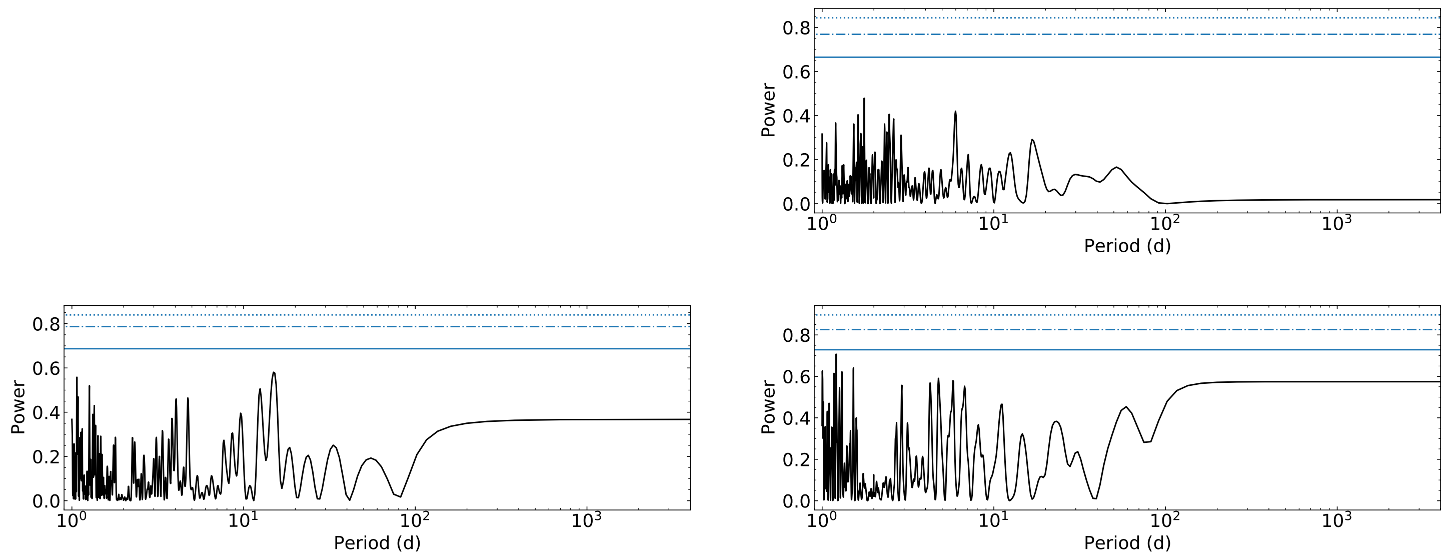


Figure 16: Same as figure 11 for 16 NARVAL spectra in the 2016 observing epoch. We do not calculate a periodogram for CaII indices since for this epoch, we calculated a CaII H index instead.

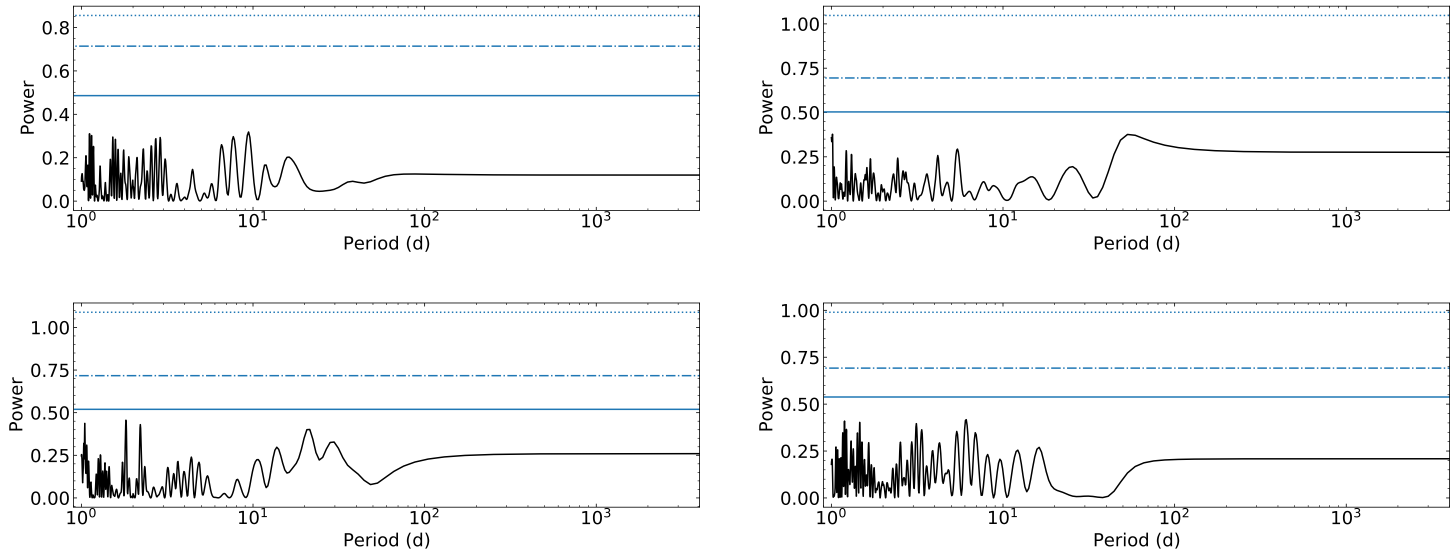


Figure 17: Same as figure 11 for 23 HARPS spectra in the 2020 observing epoch.
